# Supplementary material for: Novel techniques for efficient quantum state tomography and quantum process tomography and their experimental implementation
Source: arXiv:2401.09941 source file (2024-01-18)
Supplement: Supplementary file 2 [file appendix2.tex]

\chapter{NMR Pulse Program for Sequential Measurements}\label{SeqFID}
Below is the 2D NMR pulse program used in sequential measurements, in order to detect NCC using Eqn.(\ref{SeqFID_eq}), introduced in Sec-\ref{chapter_ncc} and Sec-\ref{mapvalue}.
\lstinputlisting[style=Matlab-editor, basicstyle=\mlttfamily\scriptsize]{SeqFID.m}
